# Supplementary material for: How Expressive are Graph Neural Networks in Recommendation?
Source: arXiv:2308.11127 source file (2023-09-15)
Supplement: Supplementary file 1 [file supplementary.tex]

\section{Supplementary Material}
\balance
\label{sec:supplementary}
